# Supplementary material for: Experimental realization of light with time separated correlations by rephasing amplified spontaneous emission
Source: arXiv:1205.0704 source file (2012-08-15)
Supplement: Supplementary file 1 [file si.pdf]

# Supplemental Material: Experimental realization of light with time separated correlations by rephasing amplified spontaneous emission


Patrick M. Ledingham,[1,*] William R. Naylor,[1,†] and Jevon J. Longdell[1,‡]

[1]*Jack Dodd Centre for Photonics and Ultra-Cold Atoms, Department of Physics, University of Otago, Dunedin, New Zealand.*



(Dated: July 10, 2012)


### Experimental Details

The energy level diagram and experimental setup are shown in Fig. A.1. An external cavity diode laser was locked to a spectral hole in a second $Tm^{3+}$:YAG crystal using a hybrid technique involving optical and electronic locking [1]. The phase of the laser was stable, with respect to coherent processes (such as photon echoes) in the thulium ions for hundreds of microseconds. The $Tm^{3+}$:YAG crystal (Scientific Materials Corp.) was held at 3 K in a pulse tube cryogenic cooler (Oxford Instruments), and measurements were taken in batches after the cooler had been turned off but before the sample had warmed up enough to affect the optical $T_2$. The crystal was cut such that the light propagated along the $\langle 1\bar{1}0 \rangle$ direction. The two level transition used was $^3H_6 \leftrightarrow {}^3H_4$ with a wavelength of 793.156 nm in air. A lens ($L_1$) of 100mm is used to focus the beam at the sample, the beam waist being 53 $\mu$m. Rabi frequencies of $\Omega/(2\pi) = 2$ MHz were achieved with driving powers of 10 mW. Light is focused on to detectors $D_1$ and $D_2$ with 50 mm lenses.

When trying to apply optical pulses with accurate pulse areas the transverse variation in intensity of a Gaussian mode is problematic. One approach is to image the light from the optical spot on the crystal onto an aperture [2] in such a way that only light from ions near the center of the spot contributes to the detected signal. The approach we take here is similar except rather than using an aperture we use the spatial filtering properties of heterodyne detection, to detect in a mode that has a smaller diameter at the sample than the driving field. The modes are illustrated in Fig. A.2.

The photodetectors used were produced in-house based on a design by Gray et al. [3] but using AD829 op-amps. The beat notes are subtracted using a RF splitter/combiner (Minicircuits), amplified with a fast saturation recovering amplifier from (Stanford SR445A), band-pass filtered around 10.7 MHz with Minicircuits components and then digitized. They are then demodulated using software to give two quadrature amplitudes as a function of time.

For the results of Fig. 1(a) the time between the two $\pi$-pulses is 100 $\mu$s, the windows of interest are 55 $\mu$s wide and are centered 47.5 $\mu$s either side of $\pi_2$. To obtain the variance, the pulse sequence is applied 2500 times at a repetition rate of 10 Hz. The 100 ms delay between shots allows enough time for total population decay between shots. Fig. 1 notes three regions of interest labeled as Vacuum, ASE and RASE. The trace has been normalized to the vacuum window. The $\pi$-pulse length is 1.6 $\mu$s. The coherence time is measured to be 13 $\mu$s using a two pulse photon echo sequence. A phase reference pulse is placed 100 $\mu$s before $\pi_1$, an order of magnitude larger than the coherence time measured. This ensures that an echo of this phase pulse does not interfere with the ASE or RASE windows of interest, the echo would appear at the same temporal location as $\pi_2$.

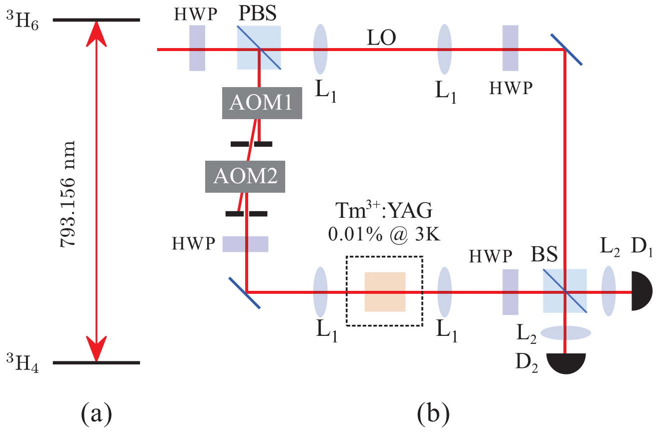


FIG. A.1: (Color online) (a) The 2 level scheme of $Tm^{3+}$:YAG. The $^3H_6 \leftrightarrow {}^3H_4$ transition has a wavelength of 793.156 nm in air. We note that there is a metastable state $^3F_4$ that is not shown here. The lifetime of this state is 10 ms. (b) Experimental setup. Laser beam passes through a polarizing beamsplitter (PBS). The probe arm is steered through two Acousto-Optic Modulators (AOM) for pulse generation, then steered toward the cryogenic $Tm^{3+}$:YAG. The signal is then combined with the local oscillator (LO) on a non-polarizing beamsplitter (BS) and sent to a balanced pair of detectors ($D_1$ and $D_2$). The two AOMs introduce a net frequency shift of 10.7 MHz between the light used to drive the $Tm^{3+}$:YAG and the local oscillator. The half waveplates (HWP) ensure that this driving light and the local oscillator have the same polarisation at the BS. The lenses $L_1$ and $L_2$ are 100 mm and 50 mm, respectively.

Referring to Fig. 2(a), there was 60 $\mu$s between $\pi_1$ and $\pi_2$, and for calculating the Duan criteria the windows are 10 $\mu$s wide centered 30 $\mu$s either side of $\pi_2$. It is

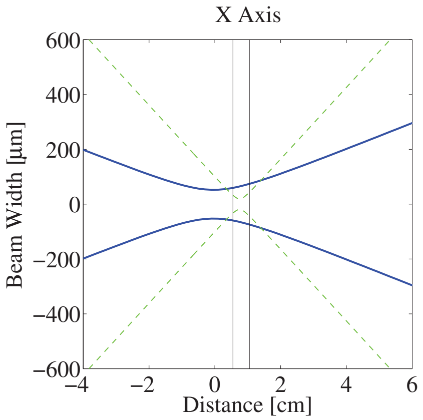


FIG. A.2: Beam size of probe and detection mode. In order to only collect light from atoms that had seen close to $\pi$-pulses, we intentionally had the interferometer mis-modematched. The beam size of the exciting light (blue solid curves) had a larger diameter in the crystal (parallel lines) than would be the case for the modematched beam (green dashed curves). The curves are a result of a fit to measurements done in the x axis of the beam. The y axis shows similar results.

noted that the coherence time for these results was 23 $\mu$s due to the crystal being colder. Due to the reduction in the magnitude of the ASE and RASE fields, this pulse sequence is applied $20 \times 10^3, 14.5 \times 10^3$ and $18.5 \times 10^3$ times at a 10 Hz repetition rate for the optical depth cases of $0.25, 0.47$ and $0.78$ respectively, to obtain statistics.

Referring to Fig. 3 the time between $\pi_1$ and $\pi_2$ was 40 $\mu$s, the temporal mode functions were Gaussian with a width of 2.5 $\mu$s placed 10.5 $\mu$s either side of $\pi_2$. Owing to the low optical depth and thus less temporal broadening of the $\pi$-pulse under propagation [4, 5], the RASE and ASE windows are allowed to be moved closer to $\pi_2$. To obtain quadrature variances, $22 \times 10^3$ shots were acquired in 44 batches of 500. Each batch had the cryo-cooler off to reduce laser noise and between the batches the cryo-cooler was restarted to cool the sample back to 3 K. The off time of the cryo-cooler was chosen such that the $T_2$ was not significantly affected. The batches were taken over a period of 2 days.

## Uncertainty in the EPR-operator variances

The left hand side of the Duan-Criteria (Eq. 3) is the variance of two operators, and each shot of our experiment gives us one measurement result for each of these two operators. The variance of this set of measurements is calculated in the standard way. The standard error ($\xi$) of the sample variance ($\sigma^2$) from $n$ samples is given by the expression [6]

$$\xi_{(\sigma^2)} = \sigma^2 \sqrt{\frac{2}{n}}. \tag{A.1}$$

The variance of $\hat{u}$, $\hat{v}$ are normalized to the vacuum region. It is thus necessary to add, in quadrature, the error in the variances $\hat{u}$, $\hat{v}$ and the vacuum region. This results in a $\sqrt{2}$ factor increase in $\xi_{(\sigma^2)}$. For the case of $\alpha l = 0.046$ we decreased the error in the vacuum region by performing statistics on 10 temporally well-separated modes immediately proceeding each shot. This results in a factor increase of $\xi_{(\sigma^2)}$ by only $\sqrt{1+\left(\frac{1}{\sqrt{10}}\right)^2} \approx 1.05$ rather than $\sqrt{2}$. Thus, one standard error in the variance is given by

$$\xi_{(\sigma^2)} = \sigma^2 \sqrt{1+\left(\frac{1}{\sqrt{10}}\right)^2} \sqrt{\frac{2}{n}}. \tag{A.2}$$

The way we have measured the vacuum level in each experimental shot should make us immune to many systematic sources of error. For example small, slow variations in the local oscillator intensity will only lead to a slight change in the weighting given to each experimental shot. The very small amount of excess classical noise that is present after the subtraction of the detector signals would be common to both the signals and vacuum and therefore also not lead to erroneous indications of entanglement.

## Inseparability Criterion

Here we describe how to obtain an analytic expression for the inseparability criterion of Duan et al. [7]. From Eq. 2 in the paper, the left hand side of Eq. 3 can be written as

$$\begin{aligned} \mathrm{var}(\hat{u}) + \mathrm{var}(\hat{v}) = & \, b \, \langle \hat{x}_1^2 \rangle + (1-b) \, \langle \hat{x}_2^2 \rangle \\ & + 2\sqrt{b\,(b-1)} \, \langle \hat{x}_1 \hat{x}_2 \rangle \\ & + b \, \langle \hat{p}_1^2 \rangle + (1-b) \, \langle \hat{p}_2^2 \rangle \\ & - 2\sqrt{b\,(b-1)} \, \langle -\hat{p}_1 \hat{p}_2 \rangle, \end{aligned} \tag{A.3}$$

where the mean of the quadratures are assumed to be zero.

From [8], one can obtain expressions for the ASE and RASE fields in terms of photonic ($\hat{a}$) and atomic ($\hat{\mathcal{D}}$) quantum operators. We state these below as

$$\hat{a}_1(l,t) = \hat{a}_1(0,t)e^{\alpha l/2} + i\alpha \int_0^l dz'\; e^{\alpha(l-z')/2}\; \hat{\mathcal{D}}_1^\dagger(z',t),$$

$$\begin{aligned}\hat{a}_2(l,t) &= \hat{a}_2(0,t)e^{-\alpha l/2} \\ &- \alpha \int_0^l dz'\; e^{\alpha(2z'-l)/2}\; \hat{a}_1^\dagger(0,-t) \\ &+ i\alpha^2 \int_0^l dz' \int_0^{z'} dz'' e^{\alpha(2z'-z''-l)/2}\; \hat{\mathcal{D}}_1(z'',-t) \\ &+ i\alpha \int_0^l dz'\; e^{\alpha(z'-l)/2}\; \hat{\mathcal{D}}_1(z',t), \qquad \text{(A.4)}\end{aligned}$$

where $\alpha l$ is the optical depth and the subscript 1(2) describes the ASE (RASE) field. It is convenient to group the creation and annihilation operators to make the following definitions:

$$\hat{a}_1(l,t) \equiv A + B^\dagger \quad \text{and} \quad \hat{a}_2(l,t) \equiv C + D^\dagger\;, \qquad \text{(A.5)}$$

where,

$$\begin{aligned} A &\equiv \hat{a}_1(0,t)e^{\alpha l/2} \\ B^\dagger &\equiv i\alpha \int_0^l dz'\; e^{\alpha(l-z')/2}\; \hat{\mathcal{D}}_1^\dagger(z',t) \\ C &\equiv \hat{a}_2(0,t)e^{-\alpha l/2} \\ &+ i\alpha^2 \int_0^l dz' \int_0^{z'} dz'' e^{\alpha(2z'-z''-l)/2}\; \hat{\mathcal{D}}_1(z'',-t) \\ &+ i\alpha \int_0^l dz'\; e^{\alpha(z'-l)/2}\; \hat{\mathcal{D}}_1(z,t) \\ D^\dagger &\equiv -\alpha \int_0^l dz'\; e^{\alpha(2z'-l)/2}\; \hat{a}_1^\dagger(0,-t)\;. \qquad \text{(A.6)}\end{aligned}$$

The functional form of the quadrature operators is the following,

$$\hat{x}_i = \hat{a}_i + \hat{a}_i^\dagger \qquad \hat{p}_i = -i\left(\hat{a}_i - \hat{a}_i^\dagger\right), \qquad \text{(A.7)}$$

where $i = \{1,2\}$. Substituting in the simplified versions of the ASE and RASE fields, it is easy to get the following for the $\hat{x}$ quadrature,

$$\begin{aligned}\langle \hat{x}_1^2\rangle &= [A,A^\dagger] + [B,B^\dagger], \\ \langle \hat{x}_2^2\rangle &= [C,C^\dagger] + [D,D^\dagger], \\ \langle \hat{x}_1\hat{x}_2\rangle &= [A,D^\dagger] + [B,C^\dagger]. \qquad \text{(A.8)}\end{aligned}$$

The terms in Eqs. A.8 are derived to get the following,

$$\begin{aligned}\langle \hat{x}_1^2\rangle &= 2\mathrm{e}^{\alpha l} - 1, \\ \langle \hat{x}_2^2\rangle &= 1 + 8\sinh^2\left(\frac{\alpha l}{2}\right), \\ \langle \hat{x}_1\hat{x}_2\rangle &= 2\left(1 - \mathrm{e}^{\alpha l}\right). \qquad \text{(A.9)}\end{aligned}$$

Identical expressions are obtained for the $\hat{p}$ quadrature by noting from Eq. A.7 that,

$$\langle \hat{x}_i^2\rangle = \langle \hat{p}_i^2\rangle \text{ and } \langle \hat{x}_i\hat{x}_j\rangle = -\langle \hat{p}_i\hat{p}_j\rangle, \qquad \text{(A.10)}$$

where $i,j = \{1,2\}$ and $i \neq j$. We can now form an analytic expression of the inseparability criterion

$$\begin{aligned}\mathrm{var}(\hat{u}) + \mathrm{var}(\hat{v}) &= 2b\;(2\mathrm{e}^{\alpha l} - 1) \\ &+ 2(1-b)\left(1 + 8\sinh^2\left(\frac{\alpha l}{2}\right)\right) \\ &+ 8\sqrt{b(1-b)}\;\left(1 - \mathrm{e}^{\alpha l}\right). \qquad \text{(A.11)}\end{aligned}$$

This expression is valid for a homodyne detector, i.e. making perfect measurements of the light quadratures. The next section explains the case for a heterodyne detector.

## Measuring the Inseparability Criterion with a Heterodyne Detector

Our experiments used heterodyne detection rather than homodyne detection mostly because of the difficulties we had in making a homodoyne detection setup that recovered quickly from the saturation caused by the two $\pi$-pulses. Here we show that the inseparability criterion of Duan et al. [7] has the same bound for heterodyne detection as for homodyne detection. Moreover, it is shown that a heterodyne detector can be used to measure entanglement, albeit less sensitively.

Heterodyne detection can be described as 'noisy' homodyne detection, simultaneously measuring both light quadratures [9]. When measuring the quadrature $\hat{x}_i$ with a heterodyne detector, one measures

$$\hat{x}_i \rightarrow \frac{\hat{x}_i + \hat{\mathrm{v}}_i}{\sqrt{2}},$$

where $i = 1$ or 2 and $\hat{\mathrm{v}}_i$ is the vacuum that enters the unused port of the 50:50 beamsplitter or equivalently the vacuum noise at $-\omega$ where $\omega$ is the heterodyning frequency. For the inseparability criterion given by Eq. 3, the variance of the operator $\hat{u}$ becomes,

$$\mathrm{var}(\hat{u}) \rightarrow b\left\langle\left(\frac{\hat{x}_1+\hat{\mathrm{v}}_1}{\sqrt{2}}\right)^2\right\rangle + (1-b)\left\langle\left(\frac{\hat{x}_2+\hat{\mathrm{v}}_2}{\sqrt{2}}\right)^2\right\rangle + 2\sqrt{b(1-b)}\left\langle\left(\frac{\hat{x}_1+\hat{\mathrm{v}}_1}{\sqrt{2}}\right)\left(\frac{\hat{x}_2+\hat{\mathrm{v}}_2}{\sqrt{2}}\right)\right\rangle$$
$$= \frac{b}{2}\left(\langle\hat{x}_1^2\rangle + \langle\hat{\mathrm{v}}_1^2\rangle + \langle\hat{x}_1\hat{\mathrm{v}}_1\rangle + \langle\hat{\mathrm{v}}_1\hat{x}_1\rangle\right) + \frac{1-b}{2}\left(\langle\hat{x}_2^2\rangle + \langle\hat{\mathrm{v}}_2^2\rangle + \langle\hat{x}_2\hat{\mathrm{v}}_2\rangle + \langle\hat{\mathrm{v}}_2\hat{x}_2\rangle\right)$$
$$+ \sqrt{b(1-b)}\Big(\langle\hat{x}_1\hat{x}_2\rangle + \langle\hat{\mathrm{v}}_1\hat{\mathrm{v}}_2\rangle + \langle\hat{x}_1\hat{\mathrm{v}}_2\rangle + \langle\hat{\mathrm{v}}_1\hat{x}_2\rangle\Big).$$

Since the variance of the vacuum is 1 and that the covariance terms between $\hat{x}$ and the vacuum equate to zero then,

$$\mathrm{var}(\hat{u}) = \frac{b}{2}\left(\langle\hat{x}_1^2\rangle + 1\right) + \frac{1-b}{2}\left(\langle\hat{x}_2^2\rangle + 1\right) + \sqrt{b(1-b)}\left(\langle\hat{x}_1\hat{x}_2\rangle\right)$$

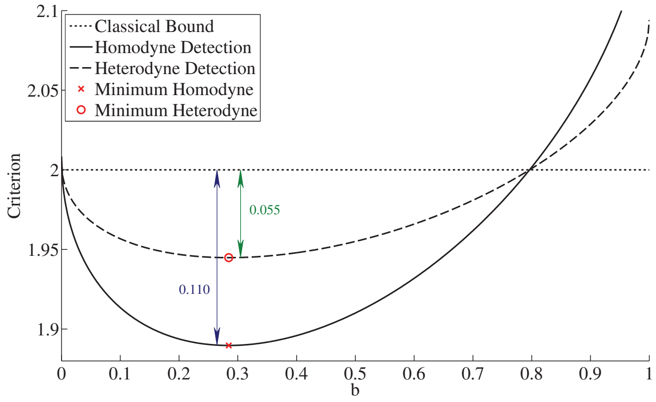


FIG. A.3: Inseparability criterion for homodyne (solid line) and heterodyne (dashed line) detection. The threshold (dotted line) is the same for both cases (see text). The curves are plotted for the experimentally relevant case of $\alpha l = 0.046$. The cross and circle indicate the minimum of the curve for homodyne and heterodyne detection respectively. Arrows indicate the 'dip' below the threshold for the minima. Heterodyne detection results in a factor of 2 less 'dip' compared to homodyne detection. This factor of 2 is the case for any point on the curve dipping below the entanglement threshold.

When comparing the above equation to the homodyne case, a factor of 2 is lost in front of the covariance term $\langle\hat{x}_1\hat{x}_2\rangle$. Hence, the correlation between the ASE and RASE fields (or equivalently, the 'dip' below the entanglement threshold) is reduced by a factor of 2 when using a heterodyne detector. Fig. A.3 shows the theoretical inseparability curves for homodyne and heterodyne detection for the experimentally relevant case of $\alpha l = 0.046$.

In a similar manner, effects such as imperfect quantum efficiency or passive loss between the sample and the detectors (for example the cryostat windows) will reduce the size of the violation of the Duan criteria but do not change the threshold.

* Present address: ICFO-Institut de Ciencies Fotoniques, Av. Carl Friedrich Gauss 3, 08860 Castelldefels (Barcelona), Spain
† Present address: Department of Physics, Norwegian University of Science and Technology, N-7491 Trondheim, Norway
‡ Electronic address: `jevon.longdell@otago.ac.nz`

[1] W. G. Farr, J. W. Tay, P. M. Ledingham, D. Korystov, and J. J. Longdell, arXiv.org (2010).
[2] J. Ruggiero, T. Chanelière, and J.-L. Le Gouët, J. Opt. Soc. Am. B **27**, 32 (2009).
[3] M. B. Gray, D. A. Shaddock, C. C. Harb, and H.-A. Bachor, Rev. Sci. Instrum. **69**, 3755 (1998).
[4] E. L. Hahn, N. S. Shiren, and S. L. McCall, Phys. Lett. **37**, 265 (1971).
[5] J. Ruggiero, T. Chaneliére, and J.-L. Le Gouët, J. Opt. Soc. Am. B **27**, 32 (2009).
[6] Y. Bar-Shalom, X. R. Li, and T. Kirubarajan, *Estimation with Applications to Tracking and Navigation* (Wiley-Interscience, 2001), ISBN 047141655X.
[7] L.-M. Duan, J. I. Cirac, P. Zoller, and E. S. Polzik, Phys. Rev. Lett. **85**, 5643 (2000).
[8] P. M. Ledingham, W. R. Naylor, J. J. Longdell, S. E. Beavan, and M. J. Sellars, Phys. Rev. A **81**, 012301 (2010).
[9] H. P. Yuen and V. W. S. Chan, Opt. Lett. **8**, 177 (1983).
